# Supplementary material for: Manipulation of the electronic structure by reversible dehydrogenation of tetra(p-hydroxyphenyl)porphyrin molecules
Source: arXiv:1403.6506 ancillary file (2014-03-25)
Supplement: Supplementary file 1 [file Supporting_Information.pdf]

# Supporting information for

## Manipulation of the electronic structure by reversible dehydrogenation of tetra(*p*-hydroxyphenyl)porphyrin molecules

Lars Smykalla[a], Pavel Shukrynau[a], Carola Mende[b], Tobias Rüffer[b], Heinrich Lang[b], Michael Hietschold[a]

[a] *Technische Universität Chemnitz, Institute of Physics, Solid Surfaces Analysis Group*
[b] *Technische Universität Chemnitz, Institute of Chemistry, Inorganic Chemistry, D-09107 Chemnitz, Germany*

---

### DFT calculation of the molecular conformation

In the gas-phase (vacuum), the porpyrin macrocycle is nearly planar for $H_2$THPP and strongly saddle-shape distorted for THPP and $H_4$THPP due to the loss of aromaticity between the pyrrole rings (Table 1). Calculations with RPBE+vdW(TS) were performed using the GPAW program.[1] For the molecules which are adsorbed on the surface no change in the conformation after deprotonation was observed by STM because the saddle-shape deformation is induced and stabilized by the molecule-substrate interaction.

Table 1: Angles of the phenyl $\alpha_{ph}$ and pyrrole $\beta_{pyr}$ rings relative to the mean plane of the molecules for the optimized geometries of $H_2$THPP, THPP and $H_4$THPP. The revised PBE exchange-correlation functional with the dispersion correction of Tkatchenko and Scheffler[2] (vdW(TS)) and the B3LYP hybrid DFT functional were used.

| | xc-functional | molecule | $\beta_{pyr}$ [°] | $\alpha_{ph}$ [°] |
|---|---|---|---|---|
| gas-phase | B3LYP | $H_2$THPP | 3 | 67 |
| gas-phase | B3LYP | THPP | 32 | 28 |
| gas-phase | RPBE+vdW(TS) | $H_2$THPP | 7 | 65 |
| gas-phase | RPBE+vdW(TS) | THPP | 26 | 29.5 |
| gas-phase | RPBE+vdW(TS) | $H_4$THPP | 26 | 30.0 |
| on Au(111)[3] | RPBE+vdW(TS) | $H_2$THPP | 23 | 32.5 |

### Interconversion events between $H_2$THPP and THPP

Spectroscopic evidence for interconversion events between **1** and **2** molecules is shown in Fig. S1. The tunneling current over time $I - t$ at constant height (open feedback loop) with the tip fixed over the center of a single molecule was measured. Large jumps of the current in $I - t$ correspond to dehydrogenation of $H_2$THPP or hydrogenation of THPP. The interconversion rate depends on the set point values of bias voltage and tunneling current. Small jumps observed in the current (Fig. S1(b)) are likely due to vibrations, an azimuthal rotation of $H_2$THPP in the structure[3] or an unstable tunneling contact after the

transfer of H atoms. Interconversion was also possible for $H_2$THPP adsorbed on Ag(110). Two characteristic current-voltage curves are shown in (Fig. S1(c)). Sudden jumps, i.e. interconversion events, occur both at negative and positive polarity (indicated by arrows).

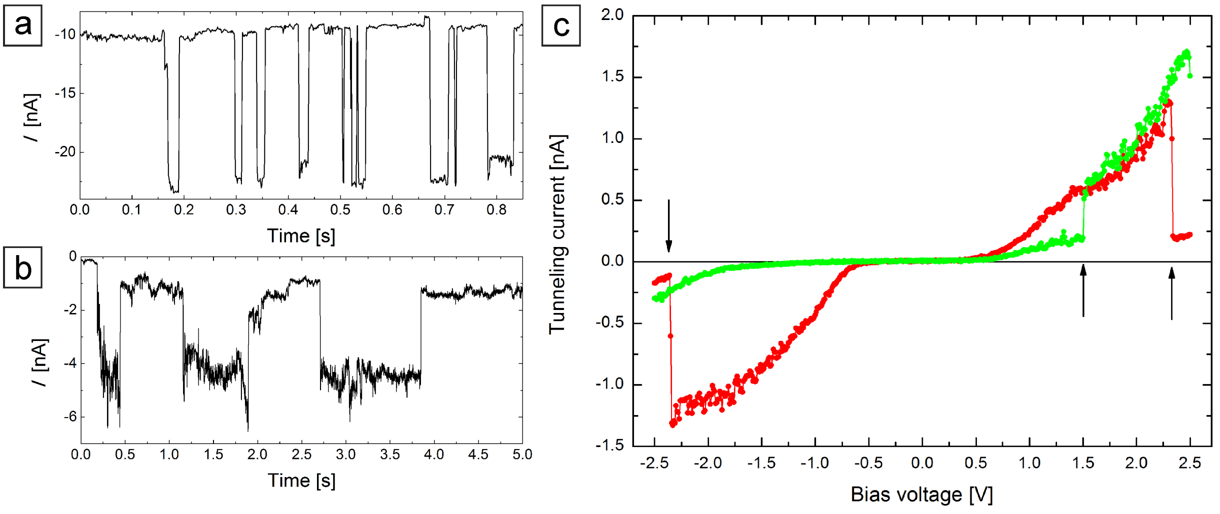


Figure S1: (a,b) Current-over-time curves for the tip positioned over one $H_2$THPP molecule at $U = -2.3$ V for two different set point currents (molecule-tip distances) before switching feedback loop off (measured at room temperature). Note that the time scale in (a) and (b) is different. (c) Current-voltage curves with jumps of the current due to interconversion events. The $I(U)$ curves were recorded for $H_2$THPP adsorbed on Ag(110).

## Single adsorbed $H_2$THPP molecules on top of the first layer

$H_2$THPP molecules on top of the first molecular layer can be clearly distinguished from appearances of **1** and **2** in the first layer by the large height difference when imaged at low bias voltage where electronic effects are small (Fig. S2). The apparent height of a $H_2$THPP molecule in STM is around 0.2 nm. The molecules atop still shows the saddle-shape deformation although it is decoupled from the Au surface by the first layer.

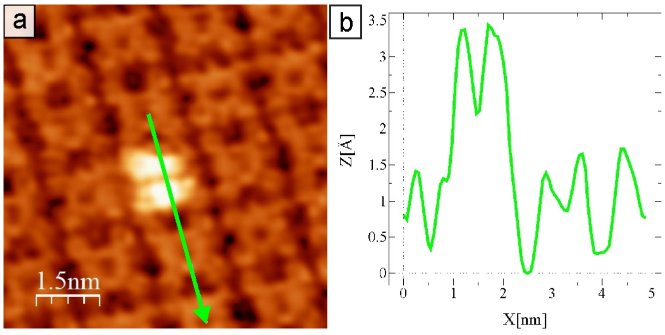


Figure S2: (a) STM image of a $H_2$THPP molecule adsorbed on top of the first molecular layer (imaging parameter: −0.5 V, 100 pA) (b) Line profile along the green arrow.

## DOS recovery from STS[4,5]:

Reasonable values of the parameters necessary for the calculation of the density of states from $(\mathbf{d}I/\mathbf{d}U)$ are chosen with the tip-sample distance $z_0 = 0.4\,\text{nm}$ and the tunneling

barrier height $\Phi = 6\,\text{eV}$. Compared to $(\mathbf{d}I/\mathbf{d}U)$ in the recovered DOS the background is removed and the occupied to empty states peak ratio changed with the intensity of the empty states notably reduced. From DFT calculations it is known that the LUMO is twofold degenerated. Thus, the recovered DOS indicates that the HOMO of **1** (red curve) is also a convolution of two molecular orbitals, while for **2** (green curve) the HOMO peak corresponds to one MO. The large peak at $-1.34$ V (also the peak at $-2.0$ V for **1**) consists then indeed of several states in general agreement with DFT calculations (5 states in DFT, see Fig. 4 of the main text). The DOS which had been calculated from the STS spectra was fitted with Voigt peak functions of identical height and width to evaluate the energetic position of molecular states in the convoluted peaks, which are summarized in Table 2.

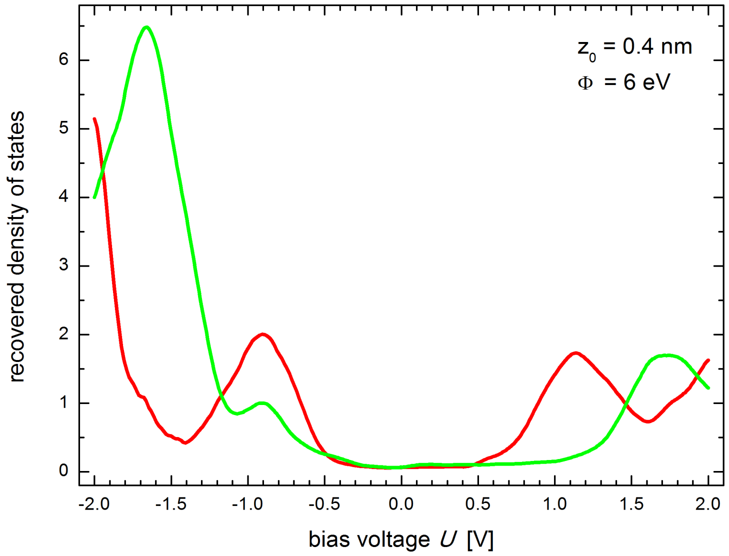


Figure S3: From STS recovered density of states for **1** (red) and **2** (green); used parameters: tip-sample distance $z_0 = 0.4$ nm, tunneling barrier height $\Phi = 6$ eV.

Table 2: Energies of molecular states fitted for the recovered DOS of form **1** and **2** of 5,10,15,20-tetra(*p*-hydroxyphenyl)porphyrin molecules on Au(111).

| Molecular orbital | $H_2$THPP | THPP |
|---|---|---|
| LUMO+2 | 1.96 V | — |
| LUMO+1 | 1.17 V | 1.81 V |
| LUMO | 1.14 V | 1.59 V |
| HOMO | -0.91 V | -0.90 V |
| HOMO-1 | -0.91 V | -1.34 V |
| HOMO-2 | -2.01 V | — |

## Materials, synthesis and characterization of $H_2$THPP

For the synthesis, the reagents were purchased from commercial suppliers. Pyrrole was distilled prior to use, while *p*-hydroxybenzaldehyde and propionic acid (99%) was used as received.

The melting point of the analytical pure sample was determined using a Mettler Toledo DSC1/700 system. TG experiments were performed with a Mettler Toledo TGA/DSC1 1100 system with an UMX1 balance. $^{1}$H NMR (500.3 MHz) and $^{13}$C {$^{1}$H} NMR (125.7 MHz) spectra were recorded with a Bruker Avance III 500 spectrometer. Chemical shifts $\delta$ are reported in ppm (parts per million) downfield from tetramethylsilane with the solvent as reference signal ($^{1}$H NMR, $CHCl_3$ $\delta$ 7.26; $^{13}$C {$^{1}$H} NMR, $CDCl_3$ $\delta$ 77.16).[6] Coupling constants $J$ are given in Hertz (Hz). Elemental analysis was measured with a Thermo FlashAE 1112 instrument. FT IR spectra were measured with a FT Nicolet IR 200 instrument (Fa. Thermo) in the range of 500 to 4000 $cm^{-1}$. The high-resolution mass spectrum was recorded with a Bruker Daltonik micrOTOF-QII spectrometer. UV/vis absorption spectra were obtained with a CECIL CE 3021 spectrophotometer in the wave length range of 200 to 800 nm.

**$H_2$THPP** was prepared according to references[7,8,9]. 4-hydroxybenzaldehyde (10.00 g, 81.86 mmol) and 5.68 ml (5.49 g, 81.86 mmol) pyrrole were added to 125 ml of propionic acid, and the resulting mixture was stirred under reflux for 1 h. After the reaction mixture was cooled to room temperature, the solvent was removed under reduced pressure. The resulting solid was washed with hot water (500 ml) and dried in a drying furnace at 130 °C. The purple powder was purified by chromatography on silica gel using acetone-light petroleum (ratio 1:1) as eluent. During slow evaporation of the solvent, $H_2$THPP (4.46 g, 67%) crystallized as purple needles.

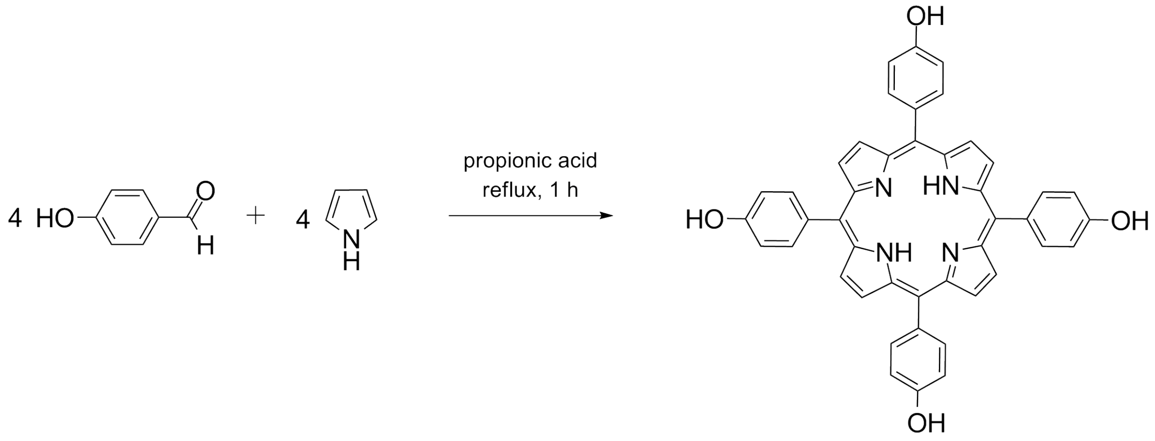

**$H_2$THPP**

Figure S4: Synthesis of 5,10,15,20-tetra($p$-hydroxyphenyl)porphyrin ($H_2$THPP).

MP: 496 °C (Decomp.). $^{1}$H NMR (500.3 MHz, $d_6$-DMSO): $\delta$ 9.93 (s, 4H), 8.87 (s, 8H), 8.00 (d, $J$ = 8.3 Hz, 8H), 7.21 (d, $J$ = 8.4 Hz, 8H), -2.87 (s, 2H). $^{13}$C {$^{1}$H} NMR (125.7 MHz, $d_6$-DMSO): $\delta$ 157.4, 135.5, 131.9, 120.0, 113.9, (the resonance signal for the pyrrole-$\alpha$-C unit could not be detected under the measurement conditions applied). Anal.Calcd for: $C_{44}H_{30}N_4O_4 \cdot 2\ H_2O$: C, 73.94; H, 4.79; N, 7.84; Found: C, 73.84; H, 4.57; N, 7.68 IR (KBr): $\tilde{v}_{max}/cm^{-1}$ 3399 (br, $\nu_{OH}$); 1605, 1587 and 1510 ($\nu_{C=C}$); 1259 ($\delta_{OH}$), 1197, 1171 (s, $\nu_{C-O}$) HRMS (ESI-TOF) $m/z$ Calcd for: $C_{44}H_{30}N_4O_4$: 679.2340; Found: 679.2378 $[M + H]^+$ UV/vis (MeOH): $\lambda_{max}$/nm ($\varepsilon$/$dm^3 \cdot mol^{-1} \cdot cm^{-1}$) 418 (386900), 517 (15400), 555 (11900), 591 (6000), 649 (6500).

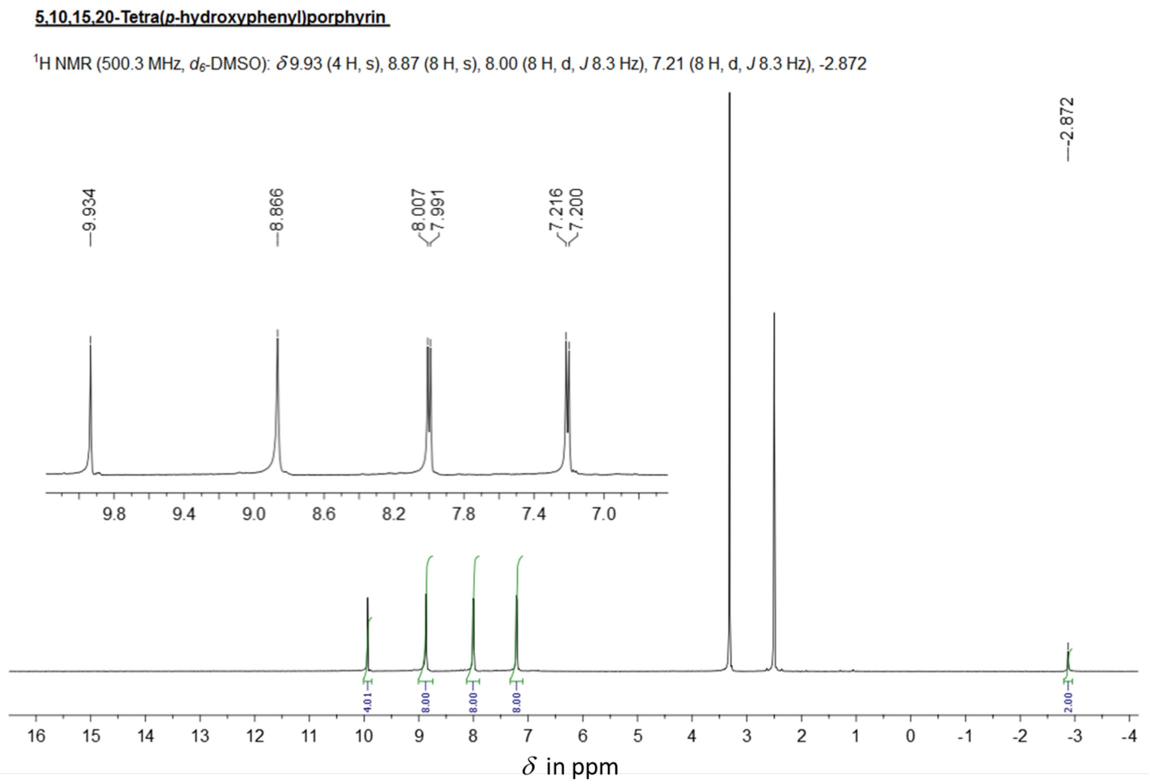


Figure S5: $^1$**H NMR** (500 MHz, $d_6$-DMSO)

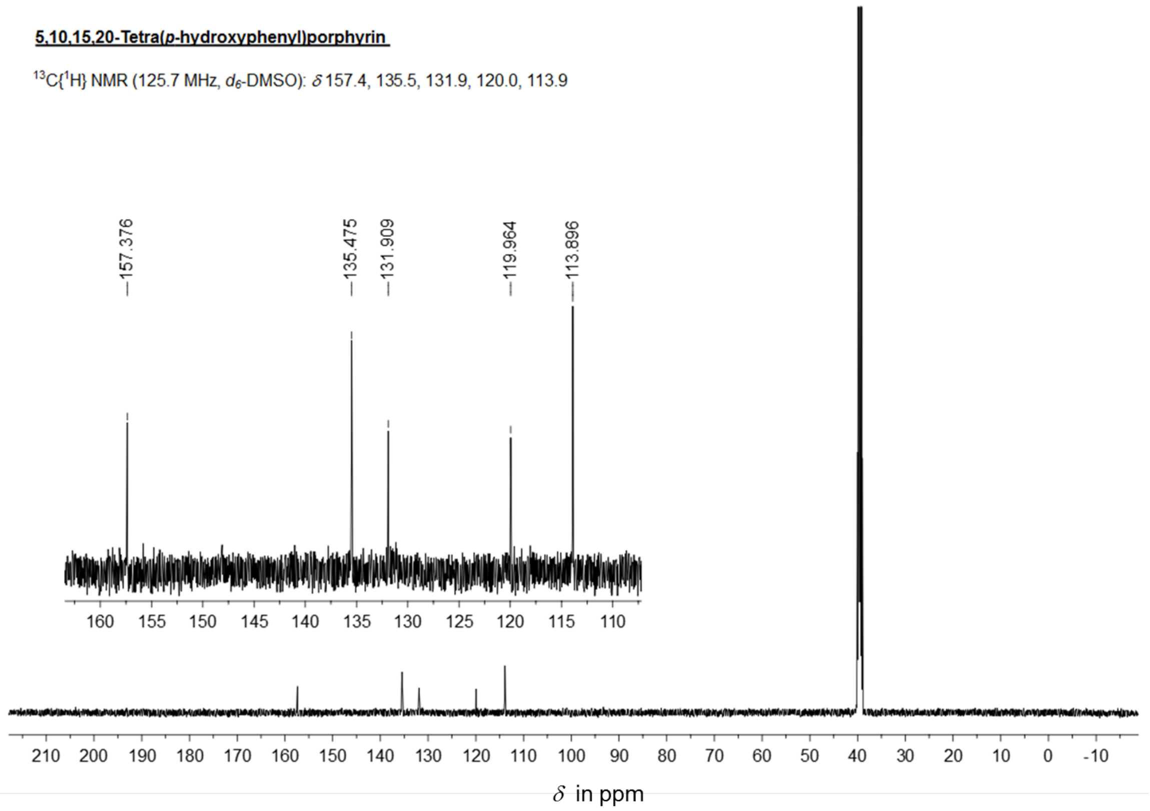


Figure S6: $^{13}$C$\{^1$H$\}$ **NMR** (125.7 MHz, $d_6$-DMSO)

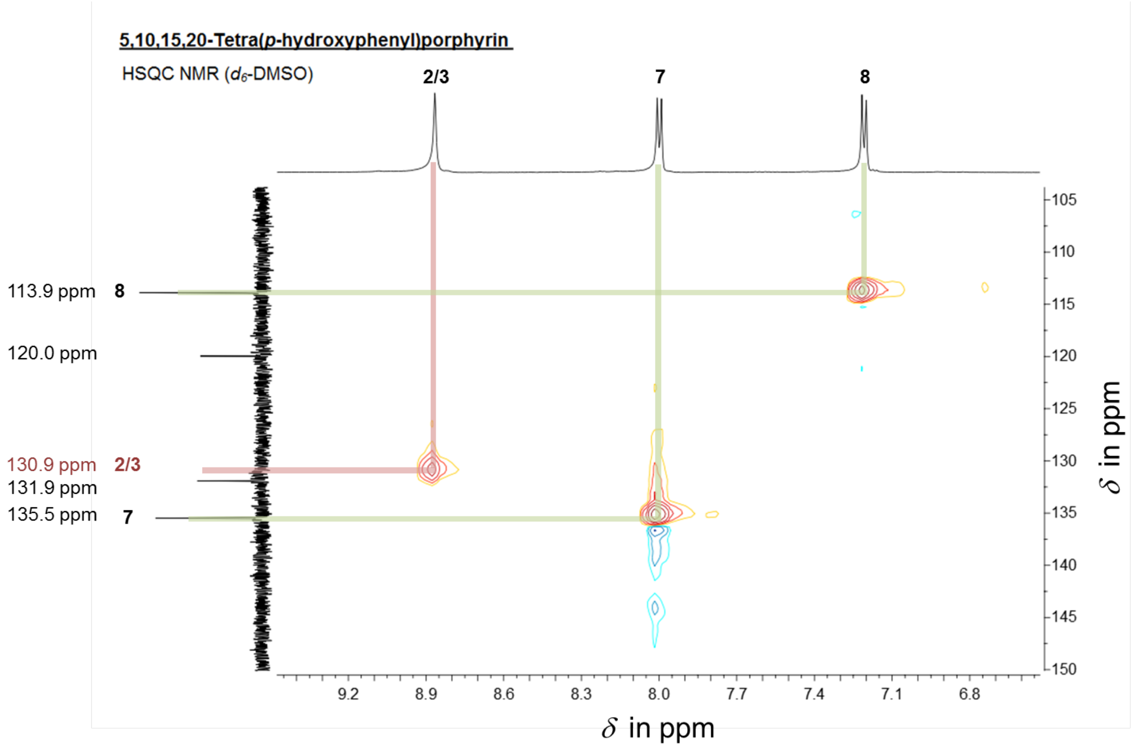


Figure S7: **HSQC NMR**

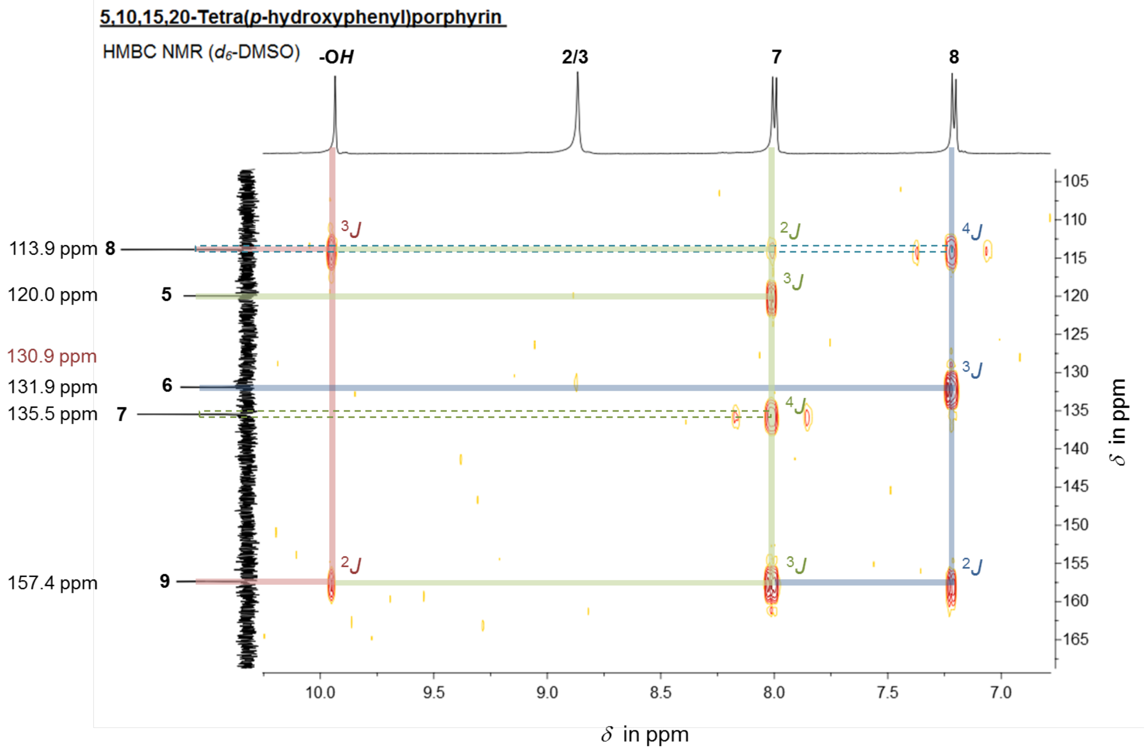


Figure S8: **HMBC NMR**

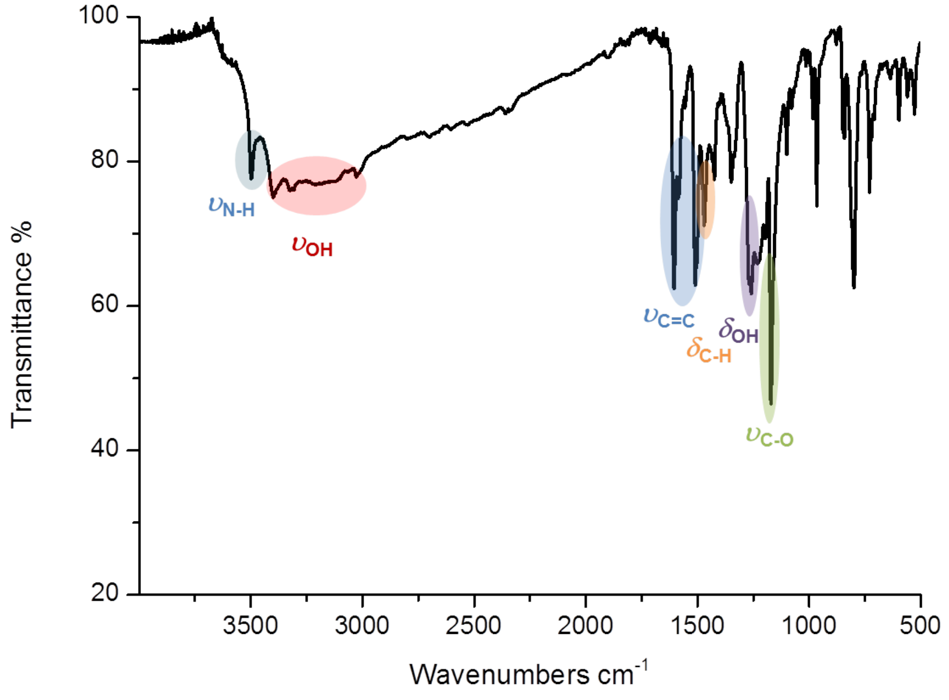


Figure S9: **IR** (KBr)

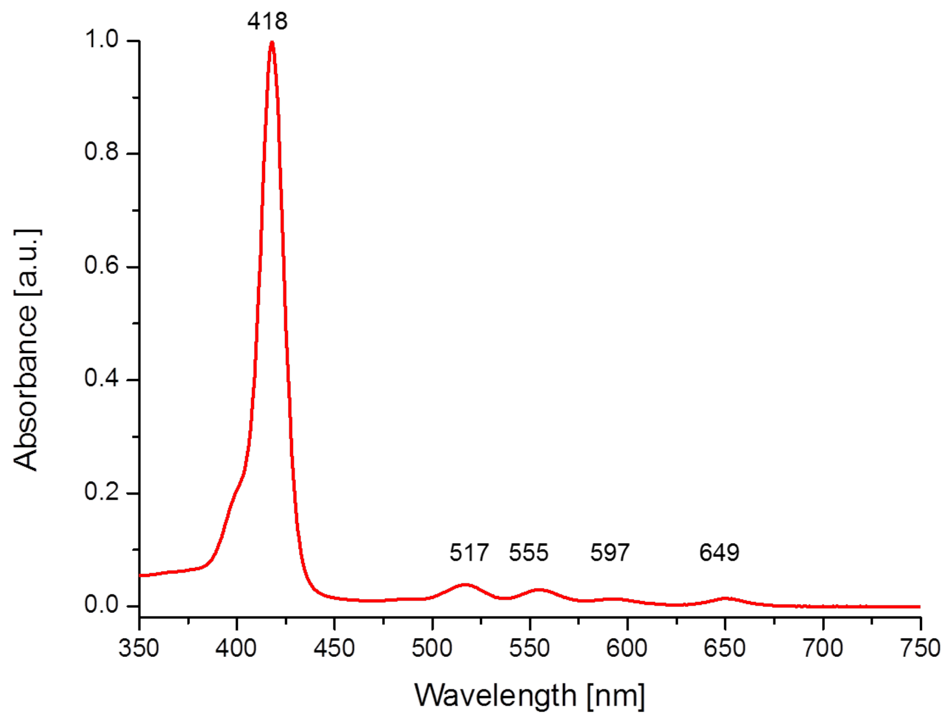


Figure S10: **UV/Vis** (MeOH)

## References


[1] J. Enkovaara, C. Rostgaard, J. J. Mortensen, J. Chen, M. Dułak, L. Ferrighi, J. Gavnholt, C. Glinsvad, V. Haikola, H. A. Hansen, H. H. Kristoffersen, M. Kuisma, A. H. Larsen, L. Lehtovaara, M. Ljungberg, O. Lopez-Acevedo, P. G. Moses, J. Ojanen, T. Olsen, V. Petzold, N. A. Romero, J. Stausholm-Møller, M. Strange, G. A. Tritsaris, M. Vanin, M. Walter, B. Hammer, H. Häkkinen, G. K. H. Madsen, R. M. Nieminen, J. K. Nørskov, M. Puska, T. T. Rantala, J. Schiøtz, K. S. Thygesen, K. W. Jacobsen, Electronic structure calculations with GPAW: a real-space implementation of the projector augmented-wave method, J. Phys.: Condens. Matter 22 (2010) 253202.

[2] A. Tkatchenko, M. Scheffler, Accurate Molecular Van Der Waals Interactions from Ground-State Electron Density and Free-Atom Reference Data, Phys. Rev. Lett. 102 (2009) 073005.

[3] L. Smykalla, P. Shukrynau, C. Mende, H. Lang, M. Hietschold, Interplay of hydrogen bonding and molecule-substrate interaction in self-assembled adlayer structures of a hydroxyphenyl-substituted porphyrin, submitted to Phys. Rev. B .

[4] B. Koslowski, C. Dietrich, A. Tschetschetkin, P. Ziemann, Evaluation of scanning tunneling spectroscopy data: Approaching a quantitative determination of the electronic density of states, Phys. Rev. B 75 (2007) 035421.

[5] C. Wagner, R. Franke, T. Fritz, Evaluation of I(V) curves in scanning tunneling spectroscopy of organic nanolayers, Phys. Rev. B 75 (2007) 235432.

[6] H. E. Gottlieb, V. Kotlyar, A. Nudelman, NMR Chemical Shifts of Common Laboratory Solvents as Trace Impurities, J. Org. Chem. 62 (1997) 7512–7515.

[7] A. D. Adler, F. R. Longo, W. Shergalis, Mechanistic investigation of porphyrin syntheses. I. Preliminary studies on ms-tetraphenylporphin, J. Am. Chem. Soc. 86 (1964) 3145–3149.

[8] A. D. Adler, F. R. Longo, J. D. Finarelli, J. Goldmacher, J. Assour, L. Korsakoff, A simplified synthesis for meso-tetraphenylporphine, J. Org. Chem. 32 (1967) 476.

[9] J. B. Kim, J. J. Leonard, F. R. Longo, A mechanistic study of the synthesis and spectral properties of meso-tetraarylporphyrin, J. Am. Chem. Soc. 94 (1972) 3986–3992.
